# Supplementary material for: Walking a Tightrope -- Evaluating Large Language Models in High-Risk Domains
Source: arXiv:2311.14966 source file (2023-11-25)
Supplement: Supplementary file 1 [file 99-appendix_eu_ai_act.tex]

%First, very rough draft. @Chia-Chien let me know if this is already too long, we can also just condense this down to a motivating paragraph in the intro. (And optionally put more details into the appendix.)
%There are 2-3 questions for Lars in the comments below, we should discuss soon if you want me to ask them or if that doesn't matter for the paper.

Evaluating LLMs in high risk domains is an important topic overall, but especially so for the future usage of LLMS within the European Union (EU). The European Union is currently preparing the EU AI act, %\footnote{See for example \url{https://digital-strategy.ec.europa.eu/en/policies/regulatory-framework-ai}, accessed June 12th 2023.},
which will regulate the AI systems deployed within the European Union in the near future.

The EU AI act foresees that AI usage will be categorized into one of four risk categories. Each risk category will have different implications on the usage and checks that needs to be run on the AI system prior to deployment. An overview for this can be found in Figure~\ref{fig:eu_ai_act}. %The four categories are: (1) Minimal risk - users have to be informed about the usage of AI and have the option to opt out; (2) Limited risk - transparency is required; (3) High risk - a conformity assessment needs to be run before an AI system is allowed to be deployed within the EU; (4) Unacceptable risk - AI is not allowed to be used for such use cases.

While the act is not yet finalized, it is already clear that at least some NLP datasets and the combined usage of LLMs will fall under the high risk category. Currently it is not yet clear if LLMs will be considered high risk by default for all use cases or if a distinction will be made based on the use case in which the LLM is applied. What is already clear and highly likely: certain use cases that employ LLMs will be considered high risk and will have to pass the EU regulation and therefore the high risk conformity assessment.

Here we explore datasets that would likely fall under the high risk use case--such as question-answering in the healthcare domain, where it would be detrimental to provided a hallucinated answer to the end user who might then risk their very life if the incorrect answer is followed. In preparation for such high risk assessments, we explore here a first step on how to evaluate LLMs under a series of different safety conscious metrics.

The need to explore how existing LLMs score with regards to the planned EU AI act was also investigated by \citet{bommasani2023eu-ai-act}. Their work focuses on all requirements, including for example the reporting of data sources and availability. One concluding remark of the study reveals an ``Absence of evaluation standards/auditing ecosystem''. We want to start addressing this shortcoming by exploring how some LLMs perform on high risk NLP datasets with regards to metrics that go beyond accuracy.

%Concretely, the below three options are under discussion:
%Option 1: FM/LLMs can be high-risk – depending on use case/use area (COM approach, in which neither GPAI nor FM are specifically addressed)

%Option 2: FM/LLMs are part of GPAI and need to fulfill high-risk requirements  (Council approach, where GPAI is specifically addressed)

%Option 3: FM/LLM treated separately and are seen as high-risk (Parliament approach, where FM are specifically addressed)
%TODO:Do we even want to discuss the 3 options or just say that something like health related NLP tasks will be high risk for sure?

%TODO: question for @Lars: what is the impact on research itself? to what degree does the act apply there?

%TODO question for @Lars: are there already any clear examples that we could give for the 4 risk categories? Do we already know any additional requirements on what checks need to be run before deployment for high risk?

%Based on the insight that at least certain use cases, such as question-answering in the healthcare domain, will most likely fall under a high risk use case within the EU, we explore in this paper a first step on evaluating LLMs for such high risk tasks under a series of different metrics.
