# Supplementary material for: Walking a Tightrope -- Evaluating Large Language Models in High-Risk Domains
Source: arXiv:2311.14966 source file (2023-11-25)
Supplement: Supplementary file 2 [file 99-appendix_old.tex]

\section{Additional Details: EU AI Act}
\label{appendix:euai}
The AI Act proposal identifies eight broad areas of high-risk AI use \cite{euai_proposal}: 
1) Biometric identification and categorisation of natural persons; 2) Management and operation of critical infrastructure; 3) Education and vocational training; 4) Employment, workers management and access to self-employment; 5) Access to and enjoyment of essential private services and public services and benefits; 6) Law enforcement; 7) Migration, asylum and border control management; and 8) Administration of justice and democratic processes. 

%\begin{enumerate}
%    \item Biometric identification and categorisation of natural persons; 
%    \item Management and operation of critical infrastructure;
%    \item Education and vocational training; 
%    \item Employment, workers management and access to self-employment;
%    \item Access to and enjoyment of essential private services and public services and benefits;
%    \item Law enforcement;
%    \item Migration, asylum and border control management;
%    \item Administration of justice and democratic processes.
%\end{enumerate}

AI and Machine Learning systems used in those high-risk areas represent high-risk AI uses and are subject to a series of mandatory requirements concerning risk management, quality management, data \& data governance, transparency \& information provision, human oversight, accuracy, robustness \& cybersecurity, as well as technical documentation and record keeping.

In the AI Act proposal, there is no specific, detailed focus on General Purpose AI systems (GPAI) or Foundation Models (FM). However, the Council of Ministers (in which all national EU member states governments are represented) and the European Parliament have addressed GPAI and FM respectively, including specific amendments.\footnote{The Council of Ministers and the European Parliament are the two EU institutions that have the shared responsibility to negotiate and decide the final Regulation text.} 

The Council of Ministers' adopted position (i.e. December 2022 \cite{euai_regulation}) on the European Commission AI Act proposal contains specific amendments in relation to rules and requirements for GPAI. The European Parliament’s adopted position (i.e. June 2023 \cite{euai_amendments}) on the AI Act proposal includes specific amendments with regard to rules and requirements for FM. It is likely that the final AI Act legal text will provide legally binding rules and requirements for GPAI and/or FM that lie somewhere in between the Council of Ministers and European Parliament’s positions on GPAI and FM respectively.\footnote{The negotiations on the AI Act/Regulation legal text are likely to be finalised by the end of 2023 resulting in its official adoption. The AI Act will probably be published in the Official Journal of the European Union during the first half of 2024. The rules and requirements will enter into force 24 months after publication.}

The Council of Ministers’ approach \cite{euai_regulation} to GPAI suggests that relevant requirements would ``apply irrespective of whether the general purpose AI system is placed on the market or put into service as a pre-trained model and whether further fine-tuning of the model is to be performed by the user of the general purpose AI system.'' (\citet{euai_regulation} p. 79)  Additionally, the Council of Ministers’ position states that GPAI systems ``which may be used as high-risk AI systems or as components of high-risk AI systems'' would have to comply with rules and requirements for high-risk AI systems (as mentioned above) (\citet{euai_regulation} p. 80). More precisely,  specific Implementing Legislation would ``specify and adapt the application of the[se] requirements […] to general-purpose AI systems in the light of their characteristics, technical feasibility, specificities of the AI value chain and of market and technological developments''.

The European Parliament’s approach to FM can be summarised as proposing that FM would have to go through a specific risk assessment to ensure compliance with health, safety fundamental rights, democracy, rule of law, the environment, etc. The obligation of such as risk assessment would be on the provider (and not the user/deployer) of the FM. The user/deployer would need to inform the provider of the deployed use case, and the provider can completely exclude various use cases from the terms of sale, however, the burden of risk assessment is clearly on the producer.  The scope of FM would cover ``a standalone model or embedded in an AI system or a product, or provided under free and open source licenses, as a service, as well as other distribution channels'' (\citet{euai_amendments} p. 199). More specifically, the European Parliament position includes, amongst others, the following requirements (Article 28b(2), page 198 of \cite{euai_amendments}) for FM providers: 
%The European Parliament position includes, amongst others, the following requirements for FM providers (Article 28b(2), page 198 of \citet{euai_amendments}):

\begin{enumerate}
    \item ``demonstrate through appropriate design, testing and analysis that the identification, the reduction and mitigation of reasonably foreseeable risks to health, safety, fundamental rights, the environment and democracy, and the rule of law prior and throughout development with appropriate methods such as with the involvement of independent experts, as well as the documentation of remaining non-mitigable risks after development'';
    \item ``process and incorporate only datasets that are subject to appropriate data governance measures for foundation models, in particular, measures to examine the suitability of the data sources and possible biases and appropriate mitigation'';
    \item ``design and develop the foundation model in order to achieve throughout its lifecycle appropriate levels of performance, predictability, interpretability, corrigibility, safety, and cybersecurity assessed through appropriate methods such as model evaluation with the involvement of independent experts, documented analysis, and extensive testing during conceptualisation, design, and development'';
    \item ``draw up extensive technical documentation and intelligible instructions for use in order to enable the downstream providers to comply with their obligations'';
    \item ``establish a quality management system to ensure and document compliance with this Article [i.e. FM related requirements], with the possibility to experiment in fulfilling this requirement''. (\citet{euai_amendments}, p. 199-200).
\end{enumerate}

Furthermore, the European Parliament position would require that providers of FM ``used in AI systems specifically intended to generate, with varying levels of autonomy, content such as complex text, images, audio, or video (``generative AI'') and providers who specialise a foundation model into generative AI system'' (\citet{euai_amendments} p. 200) ensure compliance with the following requirements (Amendment 399, Article 28 b (new) \citet{euai_amendments}):

\begin{enumerate}
    \item ``comply with the transparency obligations related to AI systems intended to interact with natural persons, i.e. ``ensure that AI systems intended to interact with natural persons are designed and developed in such a way that the AI system, the provider itself or the user informs the natural person exposed to an AI system that they are interacting with an AI system in a timely, clear and intelligible manner, unless this is obvious from the circumstances and the context of use. Where appropriate and relevant, this information shall also include which functions are AI-enabled, if there is human oversight, and who is responsible for the decision-making process'' (\citet{euai_amendments} p. 236);
    \item ``train, and where applicable, design and develop the foundation model in such a way as to ensure adequate safeguards against the generation of content in breach of Union law in line with the generally acknowledged state of the art, and without prejudice to fundamental rights, including the freedom of expression'' (\citet{euai_amendments} p. 201).
\end{enumerate}

Finally, the European Parliament position would also mandate that providers of FM have to provide certain information when registering themselves in the  forthcoming EU database for high-risk AI systems. This information would cover amongst other (Annex VIII – Section C (new) page 348 of \citet{euai_amendments}):

\begin{enumerate}
\item ``Description of the data sources used in the development of the foundational model'';
\item ``Description of the capabilities and limitations of the foundation model, including the reasonably foreseeable risks and the measures that have been taken to mitigate them as well as remaining non-mitigated risks with an explanation on the reason why they cannot be mitigated'';
\item ``Description of the training resources used by the foundation model including computing power required, training time, and other relevant information related to the size and power of the model 8. Description of the model’s performance, including on public benchmarks or state-of-the-art industry benchmarks'';
\item ``Description of the results of relevant internal and external testing and optimisation of the model'' (\citet{euai_amendments} p. 348).
\end{enumerate}

Based on these guidelines it is paramount that we develop LLMs that produce factual and safe outputs in high-risk domains as well as metrics that can reliably assess LLMs. This is particularly important because civil liability legal redress will be enhanced by the upcoming EU AI Liability Directive, which does not permit the license condition ``use at your own risk'' in the case of e.g. bodily harm.

% \section{Models and Computational Information}
% \label{appendix:computation}
% All the experiments are performed on a single Nvidia Tesla V100 GPU with 32GB VRAM and run on a GPU cluster.
% The number of parameters and the total computational budget for domain-adaptive instruction-tuning (in GPU hours) are shown in Table \ref{tab:computational}.
%\onecolumn

% \section{Details for Domain-adaptive Instruction-tuning}
% \label{appendix:hyperparameters}
% The emergence of GPT~\cite{radford-etal-2018-gpt} has led to a multitude of generative LLMs. One line of improving LLM performance has been to increase the number of model parameters~\cite{chowdhery2022palm}. However, models have become so big that they cannot easily be run and deployed on available and affordable hardware. Additionally, their computational costs are enormous. Therefore, others have focused on training smaller models (e.g., GPT-J~\citep{gpt-j}, LLaMA~\citep{touvron-etal-2023-llama}, MPT~\citep{MosaicML2023Introducing}), which are more computationally efficient and affordable, e.g. they can be run on a single GPU. In our experiments, we will rely on a series of smaller models for efficiency and cost concerns.

% For the smaller models, we use instruction-tuning~\citep{mishra-etal-2022-cross} to incorporate domain knowledge for high-risk domains. By leveraging explicit instructions during the training process, instruction-tuning has proved to enhance the model's ability for generalization~\citep{wei-etal-2022-instructiontuning} and domain adaptability~\citep{gupta-etal-2022-instructdial, wang2023codet5plus}.

% To efficiently incorporate domain knowledge, we employ QLoRA~\citep{dettmers2023qlora}, a method based on LoRA~\citep{hu-etal-2021-lora}, which compresses models using 4-bit quantization while maintaining performance parity. This reduces memory usage and enables efficient domain-adaptive instruction-tuning. The domain-adaptive instruction-tuning approach explores the capability of how smaller models can effectively adapt to high-risk domains~\citep{yunxiang2023chatdoctor}. 

% For instruction-tuning, we collect in-domain datasets for legal and medical domains. An overview of the collected datasets is shown in Table~\ref{tab:instruction_data}. To ensure the efficacy of domain-adaptive instruction-tuning approach, we follow the construction steps from~\citep{wei-etal-2022-instructiontuning}, and construct a template for each of the dataset to form the final instructions. We also explicitly control the number of instructions for both domains (13K), to have a fair comparison among approaches. To create the instructions for domain-adaptive instruction-tuning, we choose 4 datasets each for both legal and medical domains. Due to the scarcity of resources in legal domain for instructions, the medical domain data is downsampled accordingly to match the number of instances in the legal domain. We ensure that the selected number of instances for each dataset is well aligned with the tasks and sources.

% All the experiments are performed on a single Nvidia Tesla V100 GPU with 32GB VRAM and run on a GPU cluster. Table~\ref{tab:model} shows details and the computational budgets about the selected smaller models compared to the larger GPT-3.5-turbo (i.e., ChatGPT~\cite{chatgpt})\footnote{Note that we cannot do any instruction-tuning for ChatGPT as it is not possible to train the model.}. During the training process, we train for 5 epochs in batches of 64 instances. The learning rate is set to 1e-5 and the maximum sequence length is set to 1024. These settings are applied to both selected general-purpose instruction-tuned models (GPT4ALL-J, GPT4ALL-MPT)~\citep{gpt4all}. For evaluation, we set the maximum sequence length to 1024 for all compared models, and evaluate on two high-risk domains (legal, medical) with six tasks, including QA and summarization (see Table~\ref{tab:task_data})


% \input{table_instruction}
% \input{table_tasks}
% \setlength{\tabcolsep}{9.2pt}
% \begin{table*}[!]
% \centering
% \scriptsize{
% \begin{tabular}{llcccc}
% \toprule
% \textbf{Model}   & \textbf{BaseModel} &  \textbf{\# Parameters} & \textbf{Budget (in GPU hours)} & \textbf{Size} & \textbf{License}  \\\midrule
% GPT4ALL-J (tuned) & GPT-J~\citep{gpt-j} &  $\sim$3.6M & 5 hrs &   6 B      &  Apache-2.0   \\
% GPT4ALL-MPT (tuned) & MPT~\citep{MosaicML2023Introducing}  & $\sim$4.2M & 5.5 hrs &    7 B    & Apache-2.0  \\ \midrule
% GPT-3.5-turbo &  - & - & - & > 100 B& Commercial  \\
% \bottomrule
% \end{tabular}
% }
% \caption{Overview of the computational information for the domain-adaptive instruction-tuning utilizing QLoRA~\citep{dettmers2023qlora} approach, while comparing with GPT-3.5-turbo~\citep{chatgpt}.}
% \label{tab:model}
% \end{table*}
\onecolumn
%\twocolumn
%\clearpage
% \section{Details for Evaluation Metrics}
% \label{appendix:evaluation}
% We focus on two high-risk domains (legal and medical), aligned with EU AI Act domain categorization (see Figure~\ref{fig:eu_ai_act}), and evaluate 6 datasets across QA and summarization (SUM) tasks. Table~\ref{tab:task_data} shows an overview of the domain task datasets. 

% In order to evaluate the models, we utilize AuditNLG\footnote{\url{https://github.com/salesforce/AuditNLG}}, a library created to evaluate LLMs outputs from several perspectives. We focus on two metrics that we find are most relevant for high-risk domains: \textit{factuality} and \textit{safety}. 
% For the former, we use two metrics: QAFactEval \cite{fabbri-etal-2022-qafacteval}, which measures fine-grained overlap of the generated text against the ground truth, and UniEval~\citep{zhong-etal-2022-towards}, which computes over several dimensions, namely coherence, consistency, fluency and relevance. For the latter, we use Detoxify~\citep{Detoxify} and SafetyKit~\citep{dinan-etal-2022-safetykit}, which measure a model's tendencies to agree to offensive content or give the user false impressions of its capabilities as well as other safety concerns.


% \section{Overview of Models}
% \setlength{\tabcolsep}{1.6pt}
% \begin{table}[t]
% \centering
% \scriptsize{
% \begin{tabular}{llcc}
% \toprule
% \textbf{Model}                     & \textbf{BaseModel}                                     & \textbf{Size}   & \textbf{License}     \\ \midrule
% *-J  &      GPT-J~\citep{gpt-j}             &   6 B      &  Apache-2.0   \\
% %GPT4LL-Falcon &     Falcon~\citep{falcon40b}              &  7B     & Apache-2.0 \\ 
% **-MPT  &    MPT~\citep{MosaicML2023Introducing}               &    7 B    & Apache-2.0      \\ \midrule
% GPT-3.5-turbo &  - & > 100 B& Commercial\\
%                          \bottomrule
% \end{tabular}%
% }
% \vspace{-0.8em}
% \caption{Overview of the selected instruction-tuned models. * stands for GPT4ALL from~\citet{gpt4all}.}
% \vspace{-1.5em}
% \label{tab:model}
% \end{table}

%\onecolumn

\section{Evaluation on Safety}
\label{appendix:safety}
We provide the safety evaluation outcomes for each task in two high-risk domains: legal and medical, in Table~\ref{tab:results_safety_appendix} for comparisons.

\setlength{\tabcolsep}{3.0pt}
\begin{table*}[h]
\centering
\scriptsize{
\begin{tabular}{lccc ccc ccc ccc}
\toprule
 & \multicolumn{6}{c}{\textbf{Legal}} & \multicolumn{6}{c}{\textbf{Medical}} \\ \cmidrule(lr){2-7}\cmidrule(lr){8-13}
 & \multicolumn{3}{c}{\textbf{SafetyKit}} & \multicolumn{3}{c}{\textbf{Detoxify}} & \multicolumn{3}{c}{\textbf{SafetyKit}} & \multicolumn{3}{c}{\textbf{Detoxify}} \\\cmidrule(lr){2-4}\cmidrule(lr){5-7}\cmidrule(lr){8-10}\cmidrule(lr){11-13}
 & \multicolumn{1}{c}{\textbf{BillSum}} & \multicolumn{1}{c}{\textbf{CaseHold}} & \multicolumn{1}{c}{\textbf{LSE}} & \multicolumn{1}{c}{\textbf{BillSum}} & \multicolumn{1}{c}{\textbf{CaseHold}} & \multicolumn{1}{c}{\textbf{LSE}} & \multicolumn{1}{c}{\textbf{RCTSum}} & \multicolumn{1}{c}{\textbf{PubMedQA}} & \multicolumn{1}{c}{\textbf{iCliniq}} & \multicolumn{1}{c}{\textbf{RCTSum}} & \multicolumn{1}{c}{\textbf{PubMedQA}} & \multicolumn{1}{c}{\textbf{iCliniq}} \\\midrule
%\multicolumn{2}{l}{\textit{w/o instruction-tuning}} &  &  &  &  &  &  &  &  &  &  &  \\\midrule
GPT4ALL-J & 0.995 & 0.998 & 0.996 & 0.999 & 0.999 & 0.999 & 0.980 & 0.984 & 0.951 & 0.999 & 0.996 & 0.980 \\
GPT4ALL-MPT & 1.000 & 0.999 & 0.996 & 0.996 & 0.999 & 0.999 & 0.980 & 0.972 & 0.973 & 0.999  & 0.998 &  0.973 \\ \midrule
%Falcon &  &  &  &  &  &  &  &  &  &  &  &  \\ \midrule
%\multicolumn{6}{l}{\textit{with instruction-tuning }}   &  &  &  &  &  &  &  \\\midrule
GPT4ALL-J (tuned) &0.995  & 0.998 & 0.996 & 0.999 & 0.999  & 0.999 & 0.980 & 0.986  &  0.951& 0.999 &  0.996&  0.980\\
%MPT &  &  &  &  &  &  &  &  &  &  &  &  \\
GPT4ALL-MPT (tuned) & 1.000 & 0.999 & 0.996 & 0.996 & 0.999 & 0.999 & 0.980 & 0.972  &0.943  & 0.999 & 0.998 & 0.973 \\\midrule
GPT-3.5-turbo & 1.000 & 1.000 & 0.998 & 0.999 & 0.998 & 0.999 & 0.990 & 0.988 & 0.957 & 0.999 & 0.999 & 0.976\\
\bottomrule
\end{tabular}%
}
\caption{Evaluation results on safety. We use two evaluation metrics: SafetyKit~\citep{dinan-etal-2022-safetykit} and Detoxify~\citep{Detoxify}, on two high-risk domains: legal and medical.}
\label{tab:results_safety_appendix}
\end{table*}
